# Supplementary material for: Landau diamagnetism of the free electron gas as a Fermi surface effect
Source: arXiv:1807.08802 ancillary file (2018-07-27)
Supplement: Supplementary file 1 [file supplement_diamagnet.pdf]

# Landau diamagnetism of the free electron gas as a Fermi surface effect
**A. V. Nikolaev**
**SUPPLEMENTARY MATERIALS**

### APPENDIX A: ELECTRON STATES AND ENERGY OF A PARTIALLY OCCUPIED TUBE

To find the number of electron states in a partially occupied tube shown in Fig. 3 of the article, we introduce the function $y = y(x)$, Fig. 1 of the supplementary materials (SM), and integrate over volume in the cylindrical coordinates:

$$\triangle N(\Theta, \triangle\Theta) = 2\rho \int_0^{\triangle k_z} dx \int_0^{y(x)} 2\pi(k_\perp + y')dy', \tag{A1}$$

where the electron density $\rho = V/(2\pi)^3$ includes two spin polarizations and the angle span $\triangle\Theta$ is defined in Eq. (12) of the article.

Except for the polar region considered in Appendix B, and the equatorial region considered in Appendix C 1, the function $y(x)$ can be approximated by a straight line,

$$y(x) = \cot\Theta \cdot x. \tag{A2}$$

As a result of the integration over $y'$ and $x$ we then obtain

$$\triangle N = 2\pi\rho k_\perp (\triangle k_z)^2 \cot\Theta. \tag{A3}$$

In terms of $k_F$ and $\triangle k_F$ the last expression gives Eq. (13) of the article.

For the energy components $\triangle E_\perp$ and $\triangle E_z$ in respect to the components $E_\perp^0$ and $E_z^0$ of the reference energy $E_{ref} = E_\perp^0 + E_z^0$, shown in Fig. 3, 9 and 4 of the article, we obtain:

$$E_\perp^0 = \frac{\hbar^2 {k'_\perp}^2}{2m} = E_n^{aux}, \tag{A4a}$$

$$E_z^0 = \frac{\hbar^2 {k'_z}^2}{2m}. \tag{A4b}$$

Here $k'_\perp = (k_F - \triangle k_F)\sin\Theta$ and $k'_z = (k_F - \triangle k_F)\cos\Theta$. The reference energy $E_{ref} = \hbar^2(k_F - \triangle k_F)^2/2m$ represents the energy of an electron with the wave vector modulus $k_F - \triangle k_F$. In Fig. 4 of the article this energy refers to the electron energy of the state at the apex of the right angle (the $H = 0$ case).

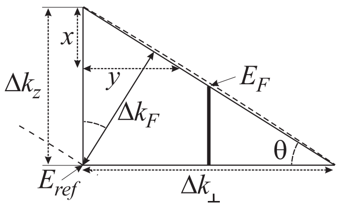


FIG. 1: The range of integration in the $(k_x, k_z)$-cross-section is approximated by the right triangle with the legs $\triangle k_\perp$, $\triangle k_z$ and $\triangle k_F$.

To find the energy component without magnetic field, $H = 0$, we calculate as in Eq. (A1), and obtain

$$\triangle E_\perp^{H=0} = 2\rho \int_0^{\triangle k_z} dx \int_0^{y(x)} dy'\, f_\perp^0(y'), \tag{A5}$$

where $y(x)$ is given by (A2) and

$$f_\perp^0(y') = \frac{\hbar^2}{2m}\left[(k_\perp + y')^2 - k_\perp^2\right] 2\pi(k_\perp + y'). \tag{A6}$$

For $\triangle E_z^{H=0}$ we get

$$\triangle E_\perp^{H=0} = 2\rho \int_0^{\triangle k_z} dx \int_0^{y(x)} dy'\, f_z^0(x, y'), \tag{A7}$$

with the function in the integral

$$f_z^0(x, y') = \frac{\hbar^2}{2m}\left[(k_z + \triangle k_z - x)^2 - k_z^2\right] 2\pi(k_\perp + y'). \tag{A8}$$

Performing the integrals (A5), (A7) and expressing the results it in terms of $k_F$ and $\triangle k_F$, Eq. (10) of the article, we arrive at

$$\triangle E_\perp^{H=0} = \frac{\hbar^2}{m}\frac{2\pi}{3}\rho\, k_F^2\, (\triangle k_F)^3 \frac{1}{\cos\Theta}, \tag{A9a}$$

$$\triangle E_z^{H=0} = \frac{\hbar^2}{m}\frac{2\pi}{3}\rho\, k_F^2\, (\triangle k_F)^3 \frac{1}{\cos\Theta}. \tag{A9b}$$

After some algebra we arrive at Eq. (19) of the article.

Now consider $\triangle E_\perp^{H\neq 0}$ and $\triangle E_z^{H\neq 0}$ in an applied magnetic field. The magnetic tube $n$ is defined in such a way that $E_\perp^0$, Eq. (A4a), coincides with $E_n^{aux}$, Eq. (5) of the article. From this it follows that the transverse electron energy component in the tube, $E_\perp^0 + \hbar\omega/2$, expressed in respect to $E_\perp^0$, leads to Eq. (20a) of the article.

For $\triangle E_z^{H\neq 0}$ we have

$$\triangle E_z^{H\neq 0} = 2\rho_z N_p \int_{\triangle k_z/2}^{\triangle k_z} dx\, f_z^H(x), \tag{A10}$$

with the integral function

$$f_z^H(x) = \frac{\hbar^2}{2m}\left[(k_z + \triangle k_z - x)^2 - k_z^2\right]. \tag{A11}$$

Having performed the integration, we obtain Eq. (20b) of the article.

## APPENDIX B: POLAR REGION

We start with finding the transverse component of the wave vector ($k_\perp$), corresponding to the zeroth tube ($n = 0$),

$$\pi k_{\perp,0}^2 = S_0^{aux} = \triangle S = \frac{2\pi}{\hbar} m\omega. \quad \text{(B1)}$$

Therefore,

$$k_{\perp,0} = \sqrt{\frac{2}{\hbar} m\omega} = \sqrt{2k_F \triangle k_F}. \quad \text{(B2)}$$

Here we have used Eq. (10) of the article. The Fermi surface intersects with the upper boundary of the zeroth tube defined by $E_{n=1}^{aux}$, Eq. (5) of the article, at the point with the coordinate $k_z$

$$k_{z,0} = \sqrt{k_F^2 - k_{\perp,0}^2} \approx k_F - \triangle k_F. \quad \text{(B3)}$$

Thus, for the zeroth tube we have

$$\triangle k_\perp = k_{\perp,0}, \quad \triangle k_z = \triangle k_F. \quad \text{(B4)}$$

For the number of active electrons in the partially occupied zeroth tube without field ($\vec{H} = 0$) we find

$$\triangle N_0 = 2\rho \int_0^{\triangle k_F} \pi y^2 dx \approx 2\pi\rho k_F (\triangle k_F)^2, \quad \text{(B5)}$$

where $y(x) = \sqrt{k_F^2 - (k_F - x)^2}$. (Here the curvature of the Fermi sphere is accounted for.) Eq. (B5) satisfies the general expression (13) of the article for $\Theta = 0$. Analogously, one can show that the other quantities (energy etc.) also follow the general consideration.

## APPENDIX C: EQUATORIAL REGION

### 1. First equatorial tube

For the angle $\triangle\Theta$ of the first equatorial tube (FET) we obtain

$$\triangle\Theta_{e,1} = \frac{\triangle k_{z,e,1}}{k_F} = \sqrt{\frac{2h}{k_F}} = \sqrt{\frac{2r\triangle k_F}{k_F}}. \quad \text{(C1)}$$

As shown in Fig. 5 of the article, we use $x = k_z$ as an independent variable changing from 0 to $\triangle k_{z,e,1}$, and consider $k_\perp$ as a function of $x$. Without magnetic field, the number of electron states in FET is given by

$$\triangle N_{e,1}^{H=0} = 2\rho\pi \int_0^{\triangle k_{z,e,1}} \left\{k_\perp^2(x) - (k_F - h)^2\right\} dx. \quad \text{(C2)}$$

Performing integration we obtain Eq. (26) of the article. With the help of (C1), we find

$$\frac{\triangle N_{e,1}^{H=0}}{\triangle\Theta_{e,1}} = \frac{8\pi r}{3} \rho\, k_F^2 \triangle k_F. \quad \text{(C3)}$$

Comparing it with the regular contribution which is obtained from Eqs. (13) and (12) of the article for $\Theta \approx \pi/2$, we arrive at Eq. (27) of the article.

For the corresponding energies (the function of integration is $y(x) = h - x^2/2k_F$), we obtain [compare with Eq. (19) of the article]

$$\frac{\triangle E_{\perp,e,1}^{H=0}}{\triangle N_{e,1}^{H=0}} = \frac{2}{5}\, r\, \hbar\omega, \quad \text{(C4a)}$$

$$\frac{\triangle E_{z,e,1}^{H=0}}{\triangle N_{e,1}^{H=0}} = \frac{1}{5}\, r\, \hbar\omega. \quad \text{(C4b)}$$

In the applied magnetic field $H$ the FET energy is a sum of two contributions: the term $\triangle E(\triangle N_{e,1}^{H\neq 0,b})$ from $\triangle N_{e,1}^{H\neq 0,b}$ and the contribution $\triangle E_{pr,1}$ from the electrons promoted from other tubes,

$$\triangle E(H \neq 0) \;=\; \triangle E_{e,1}(\triangle N_{e,1}^{H\neq 0,b}) + \triangle E_{pr,1}, \quad \text{(C5)}$$

where

$$\triangle E_{pr,1} = \left(\triangle N_{e,1}^{H=0} - \triangle N_{e,1}^{H\neq 0,b}\right) r\hbar\omega. \quad \text{(C6)}$$

Here

$$\triangle E_{e,1}(\triangle N_{e,1}^{H\neq 0,b}) = \triangle E_{\perp,e,1}^{H\neq 0,b} + \triangle E_{z,e,1}^{H\neq 0,b}, \quad \text{(C7)}$$

with

$$\frac{\triangle E_{\perp,e,1}^{H\neq 0,b}}{\triangle N_{e,1}^{H\neq 0,b}} = \frac{1}{2}\hbar\omega, \quad \text{(C8a)}$$

$$\frac{\triangle E_{z,e,1}^{H\neq 0,b}}{\triangle N_{e,1}^{H\neq 0,b}} = \frac{1}{3}\hbar\omega \left(r - \frac{1}{2}\right). \quad \text{(C8b)}$$

The regular energy contribution $\triangle E_{corr,1}$ in Eq. (32) of the article, can be written in the following form:

$$\triangle E_{corr,1} = \frac{1}{12}\hbar\omega\, \triangle N_{corr,1}, \quad \text{(C9)}$$

where

$$\triangle N_{corr,1} = 2\pi\rho k_F^2 \triangle k_F \triangle\Theta_{e,1}. \quad \text{(C10)}$$

With the help of Eqs. (C9), (C10) we obtain Eq. (33) of the article.

In computing the magnetic susceptibility, the leading term is

$$\left|\frac{\partial r}{\partial H}\right| \gg \frac{\partial\omega}{\partial H}\frac{1}{\omega}. \quad \text{(C11)}$$

Indeed, consider a magnetic field $H_0$ with the corresponding frequency $\omega_0$, at which the relation $h = 0$ and $r = 0$ are fulfilled, that is

$$E_F = \frac{\hbar^2 k_F^2}{2m} = M\hbar\omega_0, \quad \text{(C12)}$$

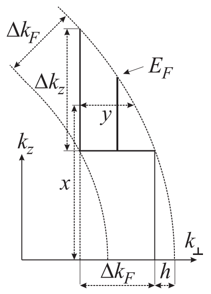


FIG. 2: The second equatorial tube and the corresponding Landau level (vertical solid line). In a magnetic field electrons from other tubes in general move to (or from) the Landau level of this tube, see text for details.

where $M$ is a big integer number. Then the lower auxiliary energy defining the first completely empty tube is $E_M^{aux} = E_F$. We shall describe this situation as having completely empty FET with the parameter $r = 0$. If we now slightly increase the magnetic field, $H' = H_0 + \delta H$, then $E_M^{aux} > E_F$. The lower FET energy boundary is defined by $E_{M-1}^{aux}$ and $0 < r < 1$. After some algebra we obtain

$$h = h_0 - \frac{m\,\delta\omega}{\hbar\, k_F}(M-1), \tag{C13}$$

where $\delta\omega = e\delta H/mc$, $h_0 = m\omega_0/\hbar k_F = \triangle k_F$. Therefore,

$$r = \frac{h}{\triangle k_F} = 1 - \frac{\delta\omega}{\omega}(M-1), \tag{C14}$$

and

$$\frac{\partial r}{\partial H} \approx -\frac{M-1}{\omega_0}\frac{\partial\omega}{\partial H} \approx \frac{e}{mc}\frac{E_F}{\hbar\omega_0^2}, \tag{C15}$$

from which it follows that $\partial r/\partial H$ is a large quantity in comparison with $\partial\omega/\partial H\,\omega$. Then for the case $a$ $(0 < r < 1/2)$ for FET we get

$$-\frac{\partial^2 f^a_{eq,1}(r)}{\partial r^2} = -\frac{5(96r^2+1)}{4r^{3/2}}. \tag{C16a}$$

In the case $b$ $(1/2 < r < 1)$

$$-\frac{\partial^2 f^b_{eq,1}(r)}{\partial r^2} = -\frac{60}{\sqrt{r-1/2}} - \frac{5}{4r^{3/2}} - 120\sqrt{r}. \tag{C16b}$$

The dependence of $\chi_{eq,1}$ from $r$ is plotted in Fig. 8 of the article.

From Eq. (C15) with the help of Eq. (2) of the article for $\omega_0$, we obtain $\partial r/\partial H \sim 1/H^2$, leading to $r \sim 1/H$.

### 2. Second equatorial tube

The second equatorial tube with all necessary parameters is shown in Fig. 2. For its description we will use the same approach which has been used for the first equatorial tube, replacing $h$ by $h + \triangle k_F$, and defining the range for $x$ from $\triangle k_{z0}\sqrt{r}$ to $\triangle k_{z0}\sqrt{1+r}$, where $\triangle k_{z0} = \sqrt{2k_F\triangle k_F}$.

Now the oscillatory part of $\chi_{eq}$, Eq. (36) of the article, is described by the function

$$\frac{\partial^2 f_{eq}(r)}{\partial r^2} = \frac{\partial^2 f_{eq,1}(r)}{\partial r^2} + \frac{\partial^2 f_{eq,2}(r)}{\partial r^2}. \tag{C17}$$

As a result for the case $a$ $(0 < r < 1/2)$ we obtain

$$-\frac{\partial^2 f^a_{eq}(r)}{\partial r^2} = \frac{60}{\sqrt{r+1/2}} - 120\sqrt{r+1} - \frac{5}{4(r+1)^{3/2}} \tag{C18a}$$

and for the case $b$ $(1/2 < r < 1)$:

$$-\frac{\partial^2 f^b_{eq}(r)}{\partial r^2} = -\frac{\partial^2 f^{(a)}_{eq}(r)}{\partial r^2} + \frac{60}{\sqrt{r-1/2}}. \tag{C18b}$$

Below we quote expressions for main quantities of the second equatorial tube. The number of electron states is

$$\triangle N^{H=0}_{e,2} = \frac{4\sqrt{2}\pi}{3}\rho(k_F\triangle k_F)^{3/2} \left(2(1+r)^{3/2} - 2r^{3/2} - 3\sqrt{r}\right), \tag{C19}$$

the angle of the $(k_x, k_z)$-cross-section is

$$\triangle\Theta_{e,2} = \frac{\triangle k_{z0}}{k_F}(\sqrt{1+r} - \sqrt{r}), \tag{C20}$$

the energy components without magnetic field are

$$\frac{\triangle E^{H=0}_{\perp,e,2}}{\hbar\omega\,\triangle N^{H=0}_{e,2}} = \frac{8(1+r)^{5/2} - 8r^{5/2} - 20r^{3/2} - 15\sqrt{r}}{10(2(1+r)^{3/2} - 2r^{3/2} - 3\sqrt{r})}, \tag{C21a}$$

$$\frac{\triangle E^{H=0}_{z,e,2}}{\hbar\omega\, N^{H=0}_{e,2}} = \frac{2}{5}\,\frac{\sqrt{1+r}(1-3r-4r^2) + 4r^{5/2} + 5r^{3/2}}{2(1+r)^{3/2} - 2r^{3/2} - 3\sqrt{r}}, \tag{C21b}$$

and finally the maximal $z$-component of the wave vector of electrons on the Landau level is

$$\delta k_F^{z,2} = \triangle k_{z0}(\sqrt{1/2+r} - \sqrt{r}). \tag{C22}$$

In the applied magnetic field $H$ the number of electron states in the tube is changed,

$$\triangle N^{H\neq 0}_{e,2} = 4\sqrt{2}\pi\rho(k_F\triangle k_F)^{3/2}\left(\sqrt{1/2+r} - \sqrt{r}\right). \tag{C23}$$

Since $\triangle N^{H\neq 0}_{e,2} > \triangle N^{H=0}_{e,2}$, a part of electron from other tubes (with the energy $\approx E_F$) moves on the Landau level of the second equatorial tube. The corresponding energy change is

$$\triangle E_{pr,2} = (\triangle N^{H=0}_{e,2} - \triangle N^{H\neq 0}_{e,2})\,\hbar\omega. \tag{C24}$$

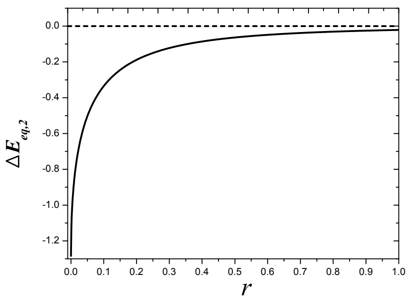


FIG. 3: The contribution to the energy $\triangle E_{eq}(r)$ from the second equatorial tube, third equatorial tube etc., see text for details.

For the energy components we obtain

$$\frac{\triangle E^{H\neq 0}_{\perp,e,2}}{\triangle N^{H\neq 0}_{e,2}} = \frac{1}{2}\hbar\omega, \tag{C25a}$$

$$\frac{\triangle E^{H\neq 0}_{z,e,2}}{\triangle N^{H\neq 0}_{e,2}} = \hbar\omega \frac{\sqrt{1/2+r}(1-4r)+4r^{3/2}}{6(\sqrt{1/2+r})-\sqrt{r})}. \tag{C25b}$$

Now we define the correction energy, Eq. (C9), to partition the energy in regular and irregular terms as in Eq. (31) of the article. For that we find $\triangle N_{corr,2}$ in correspondence with (C10), where we use (C20) for $\triangle\Theta$. We arrive at

$$\triangle E_{corr,2} = \frac{\hbar^2}{3\sqrt{2}m}\pi\rho(k_F\triangle k_F)^{5/2}\left(\sqrt{1+r}-\sqrt{r}\right). \tag{C26}$$

$\triangle E_{eq,2}$, being an additional irregular contribution to the total energy [see Eq. (37) of the article], is given by

$$\begin{aligned}\triangle E_{eq,2} &= \triangle E^{H\neq 0}_{\perp,e,2} + \triangle E^{H\neq 0}_{z,e,2} - \triangle E^{H=0}_{\perp,e,2} - \triangle E^{H=0}_{z,e,2} \\ &+\triangle E_{pr,2} - \triangle E_{corr,2}.\end{aligned} \tag{C27}$$

After some algebra, we get

$$\triangle E_{eq,2} = 2\frac{m\pi\rho}{15\sqrt{2}}\,\omega^2\sqrt{\frac{m}{\hbar}\,\omega}\; f_{eq,2}(r), \tag{C28}$$

where

$$\begin{aligned}f_{eq,2}(r) &= -\sqrt{r}(32r^2-5) - 80(1/2+r)^{3/2} \\ &+\sqrt{1+r}(27+64r+32r^2).\end{aligned} \tag{C29}$$

The function $f_{eq,2}(r)$ is plotted in Fig. 3. Notice, that $f_{eq,2}(r) < 0$ and it fast approaches zero with increasing $r$.

Notice that the inclusion of the second equatorial tube gives rise only to approximate equality between $\triangle E_{eq}(r=0)$ and $\triangle E_{eq}(r=1)$. This is because for $r=0$ we take into account only the second equatorial tube (the first is empty), while for $r=1$ we consider first and second equatorial tube. Therefore, we can further refine the accuracy by including in the equatorial region a third equatorial tube and so on. For the third, fourth etc. equatorial tubes we can still use the energy expression obtained for the second tube $\triangle E_{e,2}(r)$, but replace there the argument $r$ by $r+1$ for the third tube, $r$ by $r+2$ for the fourth tube etc. Then the oscillatory contribution can be written as

$$\triangle E_{eq} = \triangle E_{e,1}(r) + \sum_{m=0} \triangle E_{e,2}(r+m), \tag{C30}$$

where $m$ is an integer, and $\triangle E_{e,2}(r)$ is given by Eq. (C28). This implies a change of $f_{eq}(r)$,

$$f_{eq} = f_{eq,1}(r) + \sum_{m=0} f_{eq,2}(r+m), \tag{C31}$$

where the function $f_{eq,2}(r)$ is defined by (C29). However $f_{eq,2}(r)$ fast approaches zero, Fig. 3. Therefore, in practice the inclusion of third and high tubes leads only to a minor change in all expressions.
